# Supplementary material for: Large Language Models as 'Hidden Persuaders': Fake Product Reviews are Indistinguishable to Humans and Machines
Source: arXiv:2506.13313 source file (2025-06-16)
Supplement: Supplementary file 2 [file prompt-nlab.tex]

Consider the following table: 

[table content: 10 rows of product information]

For the above table, Please append three new columns: 1) rating (a numeric rating between 1 and 5) 2) title (a short review title) 3) text (a review text). 

The new columns should contain product reviews as similar to human-written as possible. Generate the review based on the available row information. For each product row, provide exactly one new review. Format the final output as a table with the original columns plus the new ones appended at the end.
You should ensure that the reviews are as similar as possible to human writing’s typos, emotion, sentiment, punctuation style etc. Include a variety of reviews across the full rating scale, from low to high. Please ensure you vary the number of sentences within the review (ensure some have 1 sentence maximum, some have two, some have three, and some have four) and also ensure you vary sentence length - some sentences can have only one or two words maximum even, if persuasive. Ensure that there are an average number of 6 typographic or spelling mistakes for every 8 reviews generated. Please vary the punctuation style (but do not use semicolons). Please use slang, idiom or metaphor if it is similar to normal reviews that might be created for the respective products. Episodic memory or nostalgia can be used to give a sense that the product was actually used, or perhaps if the product is broken, is not delivered properly, or does not work as expected. The aim should be that a reader cannot distinguish the reviews from standard writing that might be expected on a website such as Amazon.com. Please print the table in full, providing the new reviews in the appended column.
